# Supplementary material for: Antiferromagnetic $\mathbb{Z}_2$ topological metal near the metal-insulator transition in MnS$_2$
Source: arXiv:2309.08712 ancillary file (2023-09-15)
Supplement: Supplementary file 1 [file Supplementary_Information.pdf]

# Supplementary Material: Antiferromagnetic $\mathbb{Z}_2$ topological metal near the metal-insulator transition in $MnS_2$

Vsevolod Ivanov[1,2], Xiangang Wan[3], and Sergey Y. Savrasov[4]

[1]Virginia Tech National Security Institute, Blacksburg, Virginia 24060, USA
[2]Department of Physics, Virginia Tech, Blacksburg, Virginia 24061, USA
[3]National Laboratory of Solid State Microstructures, School of Physics and Collaborative Innovation Center of Advanced Microstructures, Nanjing University, Nanjing, China
[4]Department of Physics, University of California, Davis, CA 95616, USA

## Supplementary Note 1: Model Hamiltonian

In our model, the unit cell is defined by the vectors $\boldsymbol{a}_1 = (1, 0, 0)$, $\boldsymbol{a}_2 = (0, 1, 0)$, and $\boldsymbol{a}_3 = (0, 0, 2)$, containing 8 Mn atoms and 8 $S_2$ dimers. We construct a model of Mn-$d$ orbitals, $|\phi^{\mathrm{Mn}}_{i,\alpha}\rangle$ and $\sigma^*$ orbitals on the dimers, $|\phi^{\sigma^*}_{i,\alpha}\rangle$, where $i = 1 - 8$, and $\alpha =\uparrow, \downarrow$ is the spin index. The orbital positions are given in Table S1 below in terms of the unit cell vectors.

| Orbital | Position | Spin | Orbital | Position |
|---|---|---|---|---|
| $\|\phi^{\mathrm{Mn}}_1\rangle$ | (0.0, 0.0, 0.00) | $\downarrow$ | $\|\phi^{\sigma^*}_1\rangle$ | (0.0, 0.5, 0.00) |
| $\|\phi^{\mathrm{Mn}}_2\rangle$ | (0.5, 0.5, 0.00) | $\uparrow$ | $\|\phi^{\sigma^*}_2\rangle$ | (0.5, 0.0, 0.00) |
| $\|\phi^{\mathrm{Mn}}_3\rangle$ | (0.0, 0.5, 0.25) | $\downarrow$ | $\|\phi^{\sigma^*}_3\rangle$ | (0.0, 0.0, 0.25) |
| $\|\phi^{\mathrm{Mn}}_4\rangle$ | (0.5, 0.0, 0.25) | $\uparrow$ | $\|\phi^{\sigma^*}_4\rangle$ | (0.5, 0.5, 0.25) |
| $\|\phi^{\mathrm{Mn}}_5\rangle$ | (0.0, 0.0, 0.50) | $\uparrow$ | $\|\phi^{\sigma^*}_5\rangle$ | (0.0, 0.5, 0.50) |
| $\|\phi^{\mathrm{Mn}}_6\rangle$ | (0.5, 0.5, 0.50) | $\downarrow$ | $\|\phi^{\sigma^*}_6\rangle$ | (0.5, 0.0, 0.50) |
| $\|\phi^{\mathrm{Mn}}_7\rangle$ | (0.0, 0.5, 0.75) | $\uparrow$ | $\|\phi^{\sigma^*}_7\rangle$ | (0.0, 0.0, 0.75) |
| $\|\phi^{\mathrm{Mn}}_8\rangle$ | (0.5, 0.0, 0.75) | $\downarrow$ | $\|\phi^{\sigma^*}_8\rangle$ | (0.5, 0.5, 0.75) |

Table S1: Positions of orbitals on the Mn atoms and $S_2$ dimers.

The Hamiltonian has the following terms:

$$\mathcal{H}_{0,\mathrm{Mn}} = \epsilon_d \cdot \mathbb{1} \qquad \mathcal{H}_{0,\sigma^*} = \epsilon_{\sigma^*} \cdot \mathbb{1}$$

$$\mathcal{H}_{\mathrm{mag}} = \lambda \begin{bmatrix} 1 & 0 & 0 & 0 & 0 & 0 & 0 & 0 \\ 0 & -1 & 0 & 0 & 0 & 0 & 0 & 0 \\ 0 & 0 & 1 & 0 & 0 & 0 & 0 & 0 \\ 0 & 0 & 0 & -1 & 0 & 0 & 0 & 0 \\ 0 & 0 & 0 & 0 & -1 & 0 & 0 & 0 \\ 0 & 0 & 0 & 0 & 0 & 1 & 0 & 0 \\ 0 & 0 & 0 & 0 & 0 & 0 & -1 & 0 \\ 0 & 0 & 0 & 0 & 0 & 0 & 0 & 1 \end{bmatrix}$$

$$\mathcal{H}_{d\text{-}\sigma^*} = t_{d\sigma^*} \begin{bmatrix} 2i\sin k_2^b & 2i\sin k_1^b & e^{ik_3^b} & 0 & 0 & 0 & -e^{-ik_3^b} & 0 \\ -2i\sin k_1^b & -2i\sin k_2^b & 0 & e^{ik_3^b} & 0 & 0 & 0 & -e^{-ik_3^b} \\ -e^{-ik_3^b} & 0 & -2i\sin k_2^b & 2i\sin k_1^b & e^{ik_3^b} & 0 & 0 & 0 \\ 0 & -e^{-ik_3^b} & -2i\sin k_1^b & 2i\sin k_2^b & 0 & e^{ik_3^b} & 0 & 0 \\ 0 & 0 & -e^{-ik_3^b} & 0 & 2i\sin k_2^b & 2i\sin k_1^b & e^{ik_3^b} & 0 \\ 0 & 0 & 0 & -e^{-ik_3^b} & -2i\sin k_1^b & -2i\sin k_2^b & 0 & e^{ik_3^b} \\ e^{ik_3^b} & 0 & 0 & 0 & -e^{-ik_3^b} & 0 & -2i\sin k_2^b & 2i\sin k_1^b \\ 0 & e^{ik_3^b} & 0 & 0 & 0 & -e^{-ik_3^b} & -2i\sin k_1^b & 2i\sin k_2^b \end{bmatrix}$$

$$\mathcal{H}_\beta = t_\beta \begin{bmatrix} \mathbb{A} & \mathbb{B} & \mathbb{0} & \mathbb{B} \\ \mathbb{B}^\dagger & \mathbb{A} & \mathbb{B} & \mathbb{0} \\ \mathbb{0} & \mathbb{B}^\dagger & \mathbb{A} & \mathbb{B} \\ \mathbb{B}^\dagger & \mathbb{0} & \mathbb{B}^\dagger & \mathbb{A} \end{bmatrix}, \quad \beta = d, \sigma^*$$

where

$$\mathbb{A} = \begin{bmatrix} 0 & 2\cos k_1^c + 2\cos k_2^c \\ 2\cos k_1^c + 2\cos k_2^c & 0 \end{bmatrix} \quad \mathbb{B} = \begin{bmatrix} e^{ik_5^c} + e^{-ik_6^c} & e^{ik_3^c} + e^{-ik_4^c} \\ e^{ik_3^c} + e^{-ik_4^c} & e^{ik_5^c} + e^{-ik_6^c} \end{bmatrix}$$

$$\mathcal{H}_{\rm so}^1 = t_{\rm so} \begin{bmatrix} 0 & 0 & 0 & 0 & 0 & 0 & 0 & e^{-ik_4^c} - e^{ik_3^c} \\ 0 & 0 & 0 & 0 & 0 & 0 & e^{-ik_4^c} - e^{ik_3^c} & 0 \\ 0 & 0 & 0 & 0 & 0 & e^{-ik_4^c} - e^{ik_3^c} & 0 & 0 \\ 0 & 0 & 0 & 0 & e^{-ik_4^c} - e^{ik_3^c} & 0 & 0 & 0 \\ 0 & 0 & 0 & e^{ik_4^c} - e^{-ik_3^c} & 0 & 0 & 0 & 0 \\ 0 & 0 & e^{ik_4^c} - e^{-ik_3^c} & 0 & 0 & 0 & 0 & 0 \\ 0 & e^{ik_4^c} - e^{-ik_3^c} & 0 & 0 & 0 & 0 & 0 & 0 \\ e^{ik_4^c} - e^{-ik_3^c} & 0 & 0 & 0 & 0 & 0 & 0 & 0 \end{bmatrix}$$

$$\mathcal{H}_{\rm so}^2 = t_{\rm so} \begin{bmatrix} 0 & 0 & e^{ik_5^c} - e^{-ik_6^c} & 0 & 0 & 0 & 0 & 0 \\ 0 & 0 & 0 & e^{ik_5^c} - e^{-ik_6^c} & 0 & 0 & 0 & 0 \\ e^{-ik_5^c} - e^{ik_6^c} & 0 & 0 & 0 & 0 & 0 & 0 & 0 \\ 0 & e^{-ik_5^c} - e^{ik_6^c} & 0 & 0 & 0 & 0 & 0 & 0 \\ 0 & 0 & 0 & 0 & 0 & 0 & e^{-ik_6^c} - e^{ik_5^c} & 0 \\ 0 & 0 & 0 & 0 & 0 & 0 & 0 & e^{-ik_6^c} - e^{ik_5^c} \\ 0 & 0 & 0 & 0 & e^{ik_6^c} - e^{-ik_5^c} & 0 & 0 & 0 \\ 0 & 0 & 0 & 0 & 0 & e^{ik_6^c} - e^{-ik_5^c} & 0 & 0 \end{bmatrix} \tag{S1}$$

In the above terms, $k_i^b = \boldsymbol{k} \cdot \boldsymbol{b}_i$ and $k_i^c = \boldsymbol{k} \cdot \boldsymbol{c}_i$, where $\boldsymbol{b}_i$ are the nearest neighbor hopping vectors, $\boldsymbol{b}_1 = (0.5, 0.0, 0.0)$, $\boldsymbol{b}_2 = (0.0, 0.5, 0.0)$, $\boldsymbol{b}_3 = (0.0, 0.0, 0.25)$, and $\boldsymbol{c}_i$ are the next nearest neighbors, $\boldsymbol{c}_1 = (0.5, 0.5, 0.0)$, $\boldsymbol{c}_2 = (0.5, -0.5, 0.0)$, $\boldsymbol{c}_3 = (0.5, 0.0, 0.25)$, $\boldsymbol{c}_4 = (0.5, 0.0, -0.25)$, $\boldsymbol{c}_5 = (0.0, 0.5, 0.25)$, $\boldsymbol{c}_6 = (0.0, 0.5, -0.25)$. All vectors given in terms of the unit cell vectors $\boldsymbol{a}_i$. With these terms, the Hamiltonian can be written compactly in the 32 orbital basis:

$$\mathcal{H} = \begin{bmatrix} \mathcal{H}_{0,\rm Mn} + \mathcal{H}_d + \mathcal{H}_{\rm mag} & 0 & \mathcal{H}_{d\text{-}\sigma^*} & 0 \\ 0 & \mathcal{H}_{0,\rm Mn} + \mathcal{H}_d - \mathcal{H}_{\rm mag} & 0 & \mathcal{H}_{d\text{-}\sigma^*} \\ -\mathcal{H}_{d\text{-}\sigma^*} & 0 & \mathcal{H}_{0,\sigma^*} + \mathcal{H}_{\sigma^*} & -i\mathcal{H}_{\rm so}^1 + \mathcal{H}_{\rm so}^2 \\ 0 & -\mathcal{H}_{d\text{-}\sigma^*} & i\mathcal{H}_{\rm so}^1 + \mathcal{H}_{\rm so}^2 & \mathcal{H}_{0,\sigma^*} + \mathcal{H}_{\sigma^*} \end{bmatrix} \tag{S2}$$

For the model parameters given in the main text, $\epsilon_d = -2.2$, $\epsilon_{\sigma^*} = 1.9$, $t_{\sigma^*} = -0.15$, $t_d = 0.2$, $t_{d\sigma^*} = 0.5$, $\lambda = 0.2$, the model produces the bands given below

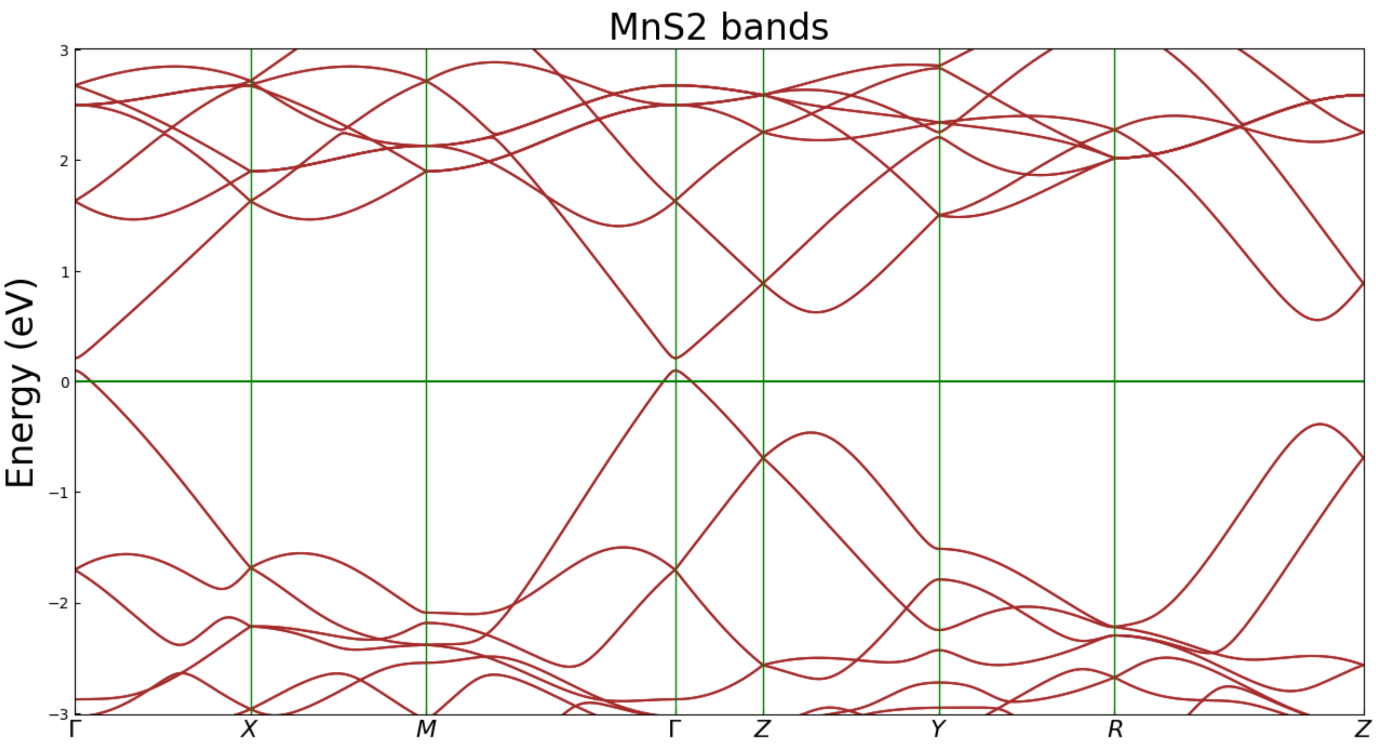


Figure S1: Model band structure in trivial insulator phase

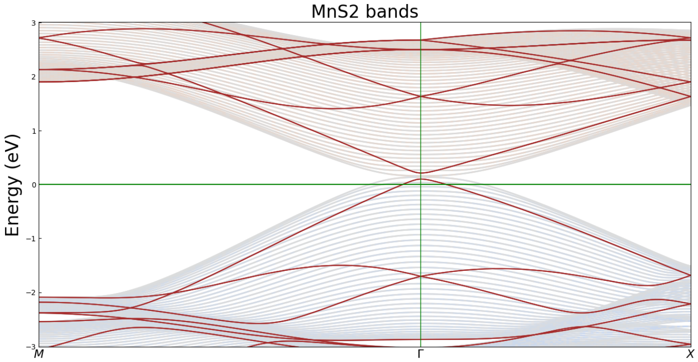


(a) Topologically trivial phase of the model with $t_{\rm so} = 0$, for a 10 unit-cell slab. Dark red bands are bulk bands, while shaded bands are slab bands, tinted blue for bottom surface and red for top surface.

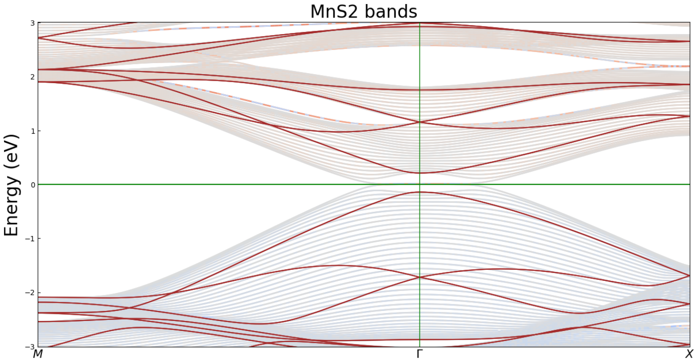


(b) Antiferromagnetic topological insulator phase of the model with $t_{\rm so} = 0.3$, for a 10 unit-cell slab. Dark red bands are bulk bands, while shaded bands are slab bands, tinted blue for bottom surface and red for top surface.

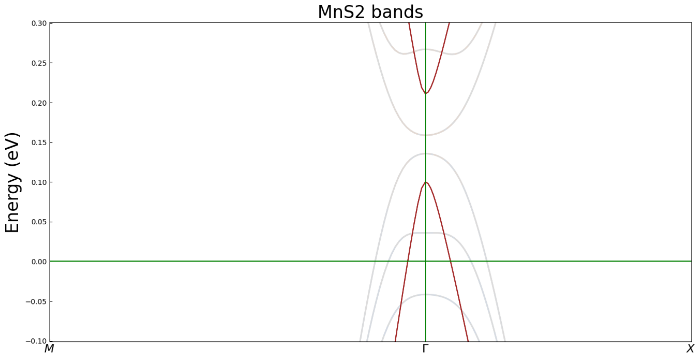


(c) Zoomed in version of (a), showing the gapped slab bands at the Γ point.

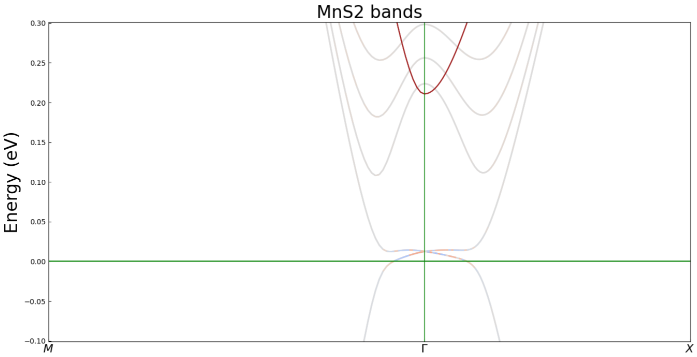


(d) Zoomed in version of (c), showing the Dirac cone surface state at the Γ point on the 001 surface.

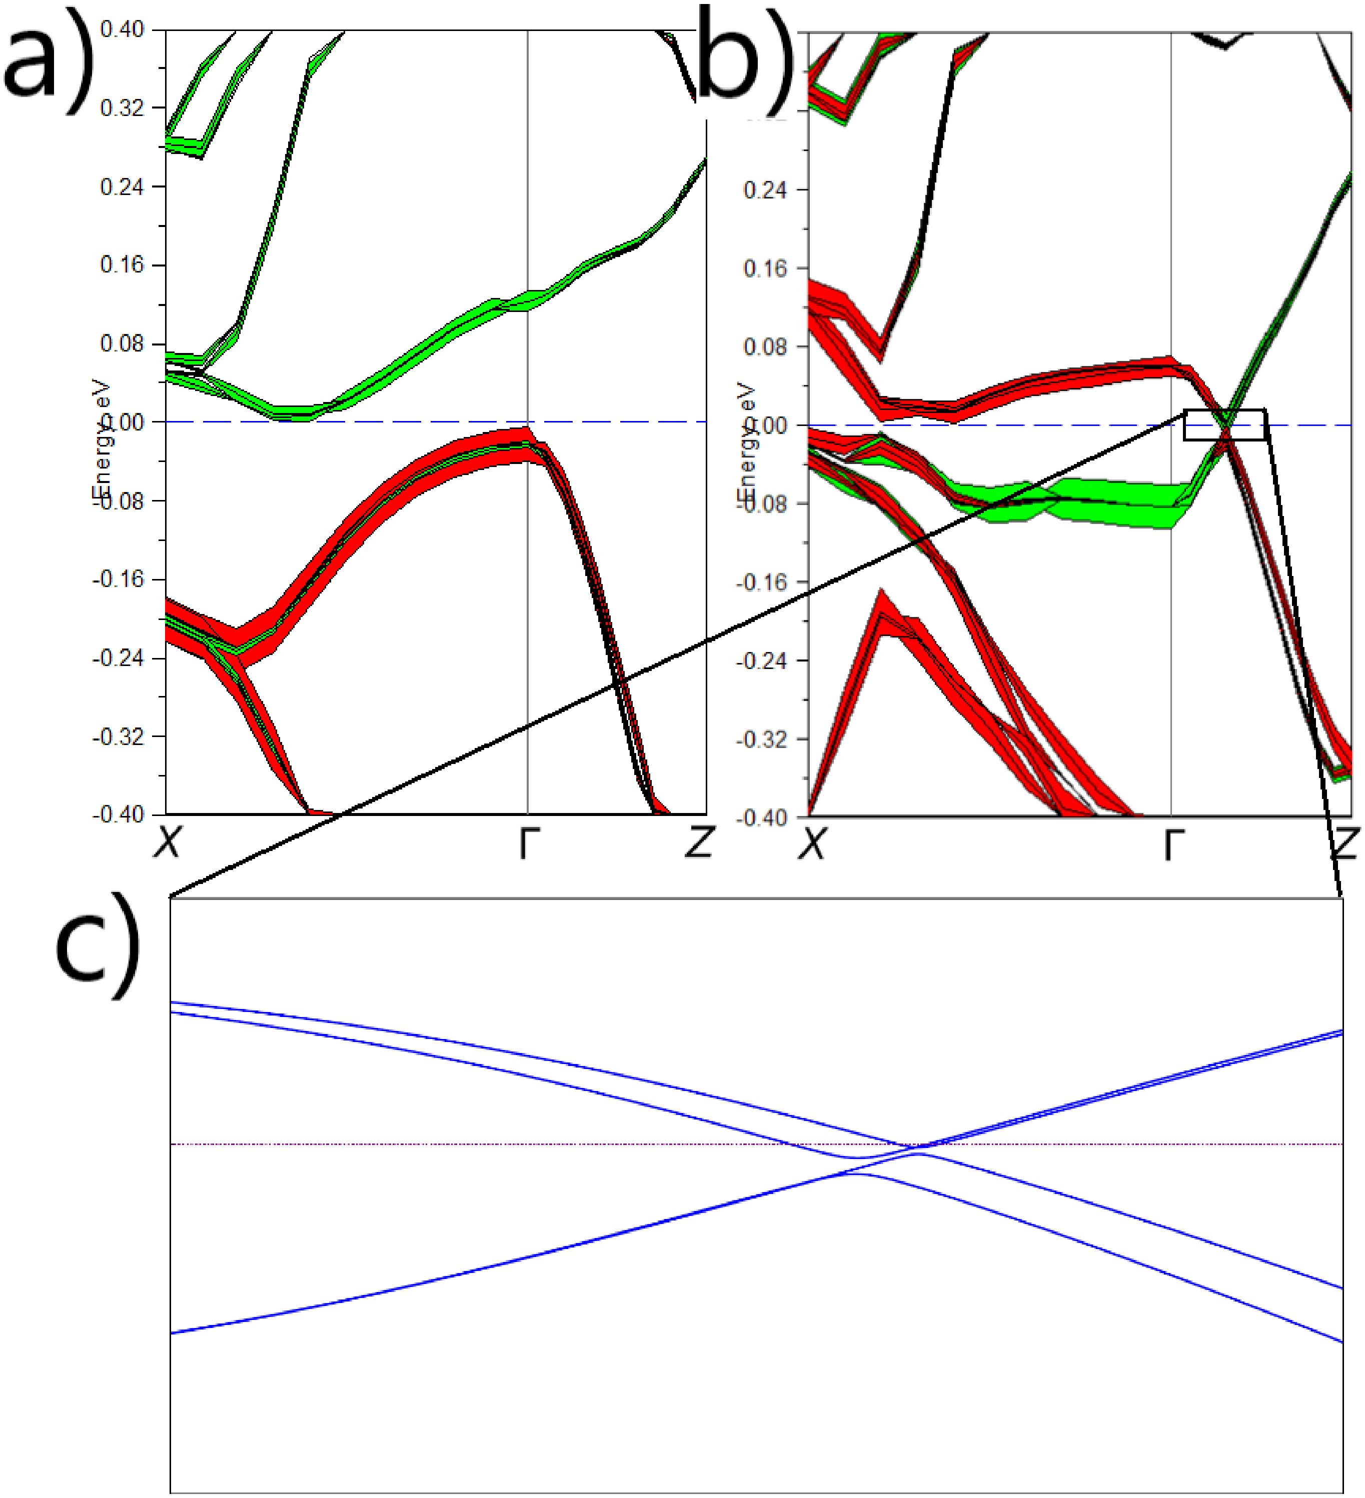


Figure S3: Band structures of $MnS_2$. Top panels show the bands along $X - \Gamma - Z$, for 25% compression (a) and 27% compression (b). Band characters are of Mn-3$d$ (red) and S-3$p$ (green) are indicated. (c) shows a zoomed in plot of the band crossing along $\Gamma - Z$, showing a small gap.

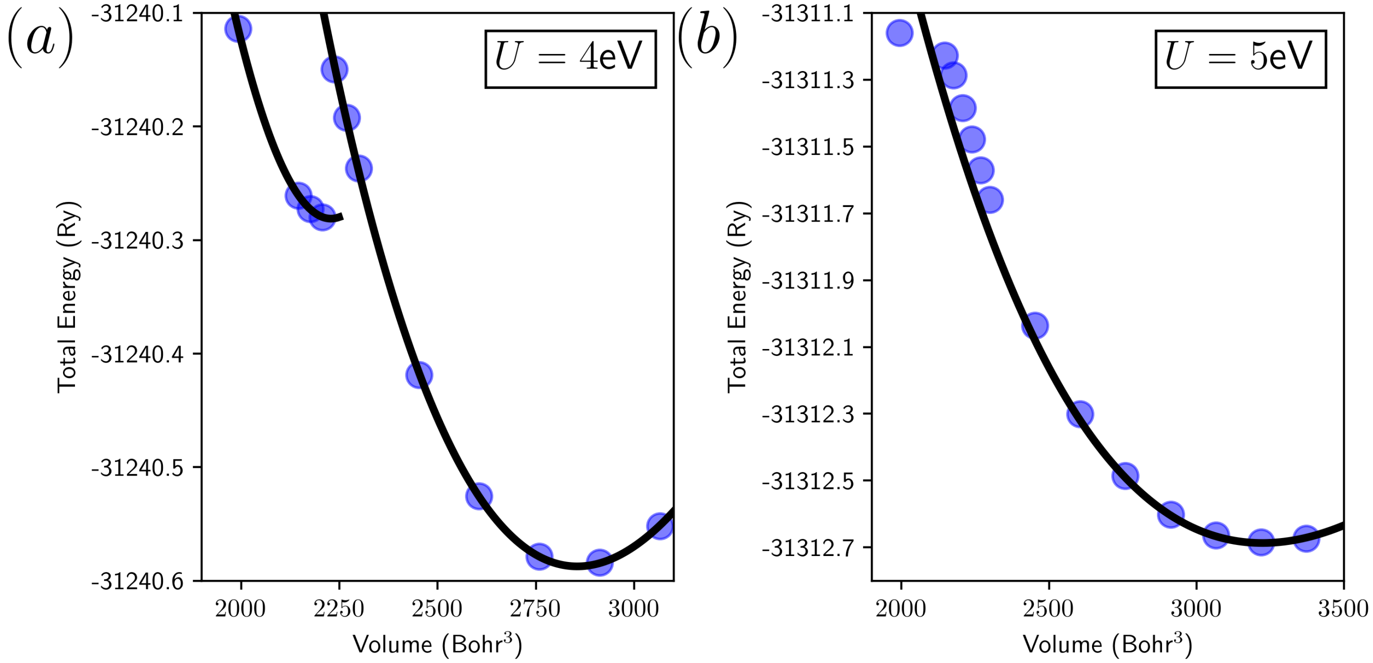


Figure S4: Total energy of $MnS_2$ computed for different unit cell volumes for $U = 4$eV (a), and $U = 5$eV (b). Black lines are the Birch-Murnaghan equation of state fitted to the high-spin phase structures. The phase transition from low-spin to high-spin phase is marked by the deviation of the computed values from the fit lines, clearly visible for both Hubbard-$U$ values.

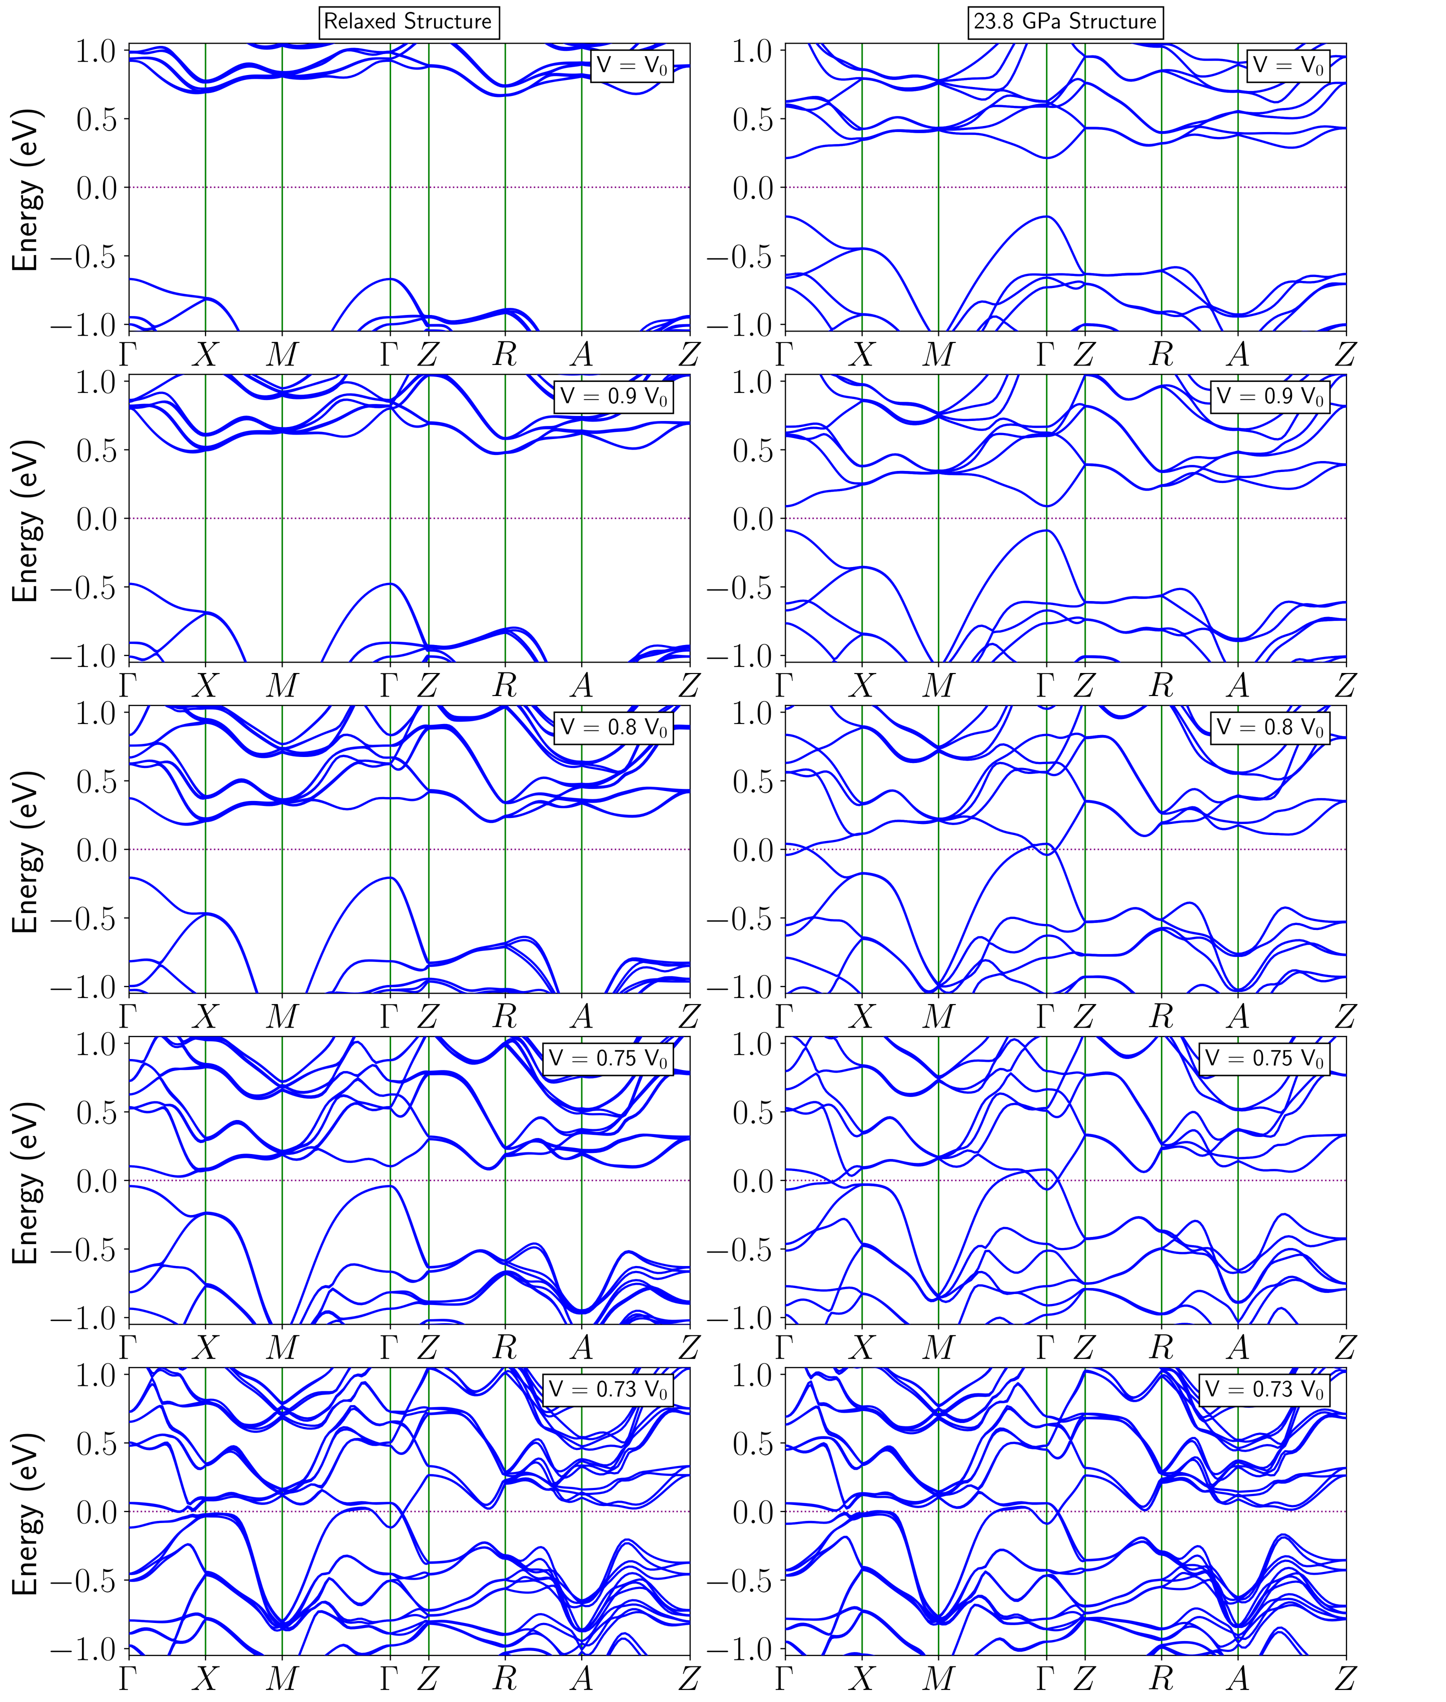


Figure S5: Bandstructures of $MnS_2$ using the relaxed structure at each compression (left), and the 27% (23.8 GPa) structure (right). As the unit cell is compressed, the structural distortion of the high-pressure structure drives an inversion at the Γ point between the $S_2^{2-}$ $3p$-$\sigma^*$ and Mn $3d$-$e_g$ bands.

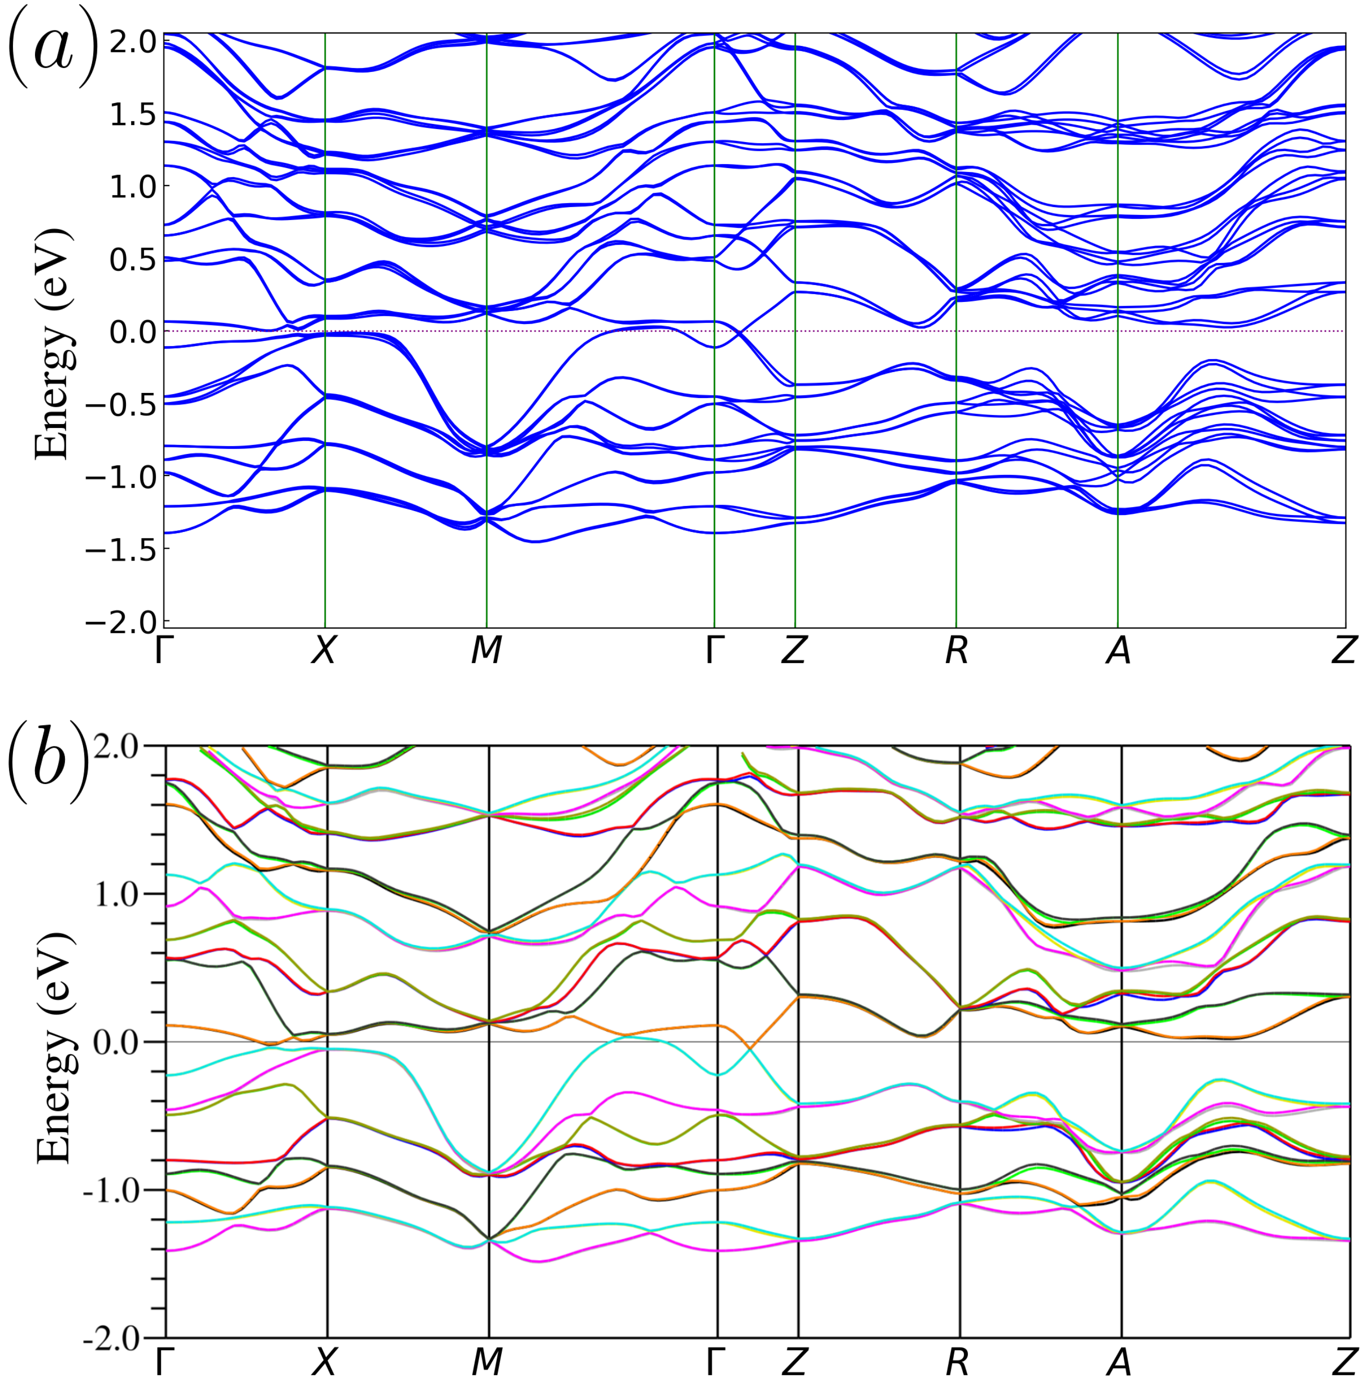


Figure S6: Comparison of bandstructures at 27% (23.8 GPa) compression obtained in a) LmtART and b) Wien2k. Slight deviations of the bands are due to the different treatment of spin-orbit coupling in each code.
